# Supplementary material for: DeepOPF: A Feasibility-Optimized Deep Neural Network Approach for AC Optimal Power Flow Problems
Source: arXiv:2007.01002 source file (2022-07-01)
Supplement: Supplementary file 1 [file appendix_old.tex]

\begin{appendices}
% \section{A 2-bus Example} \label{apx:2busexample}
% We consider a 2-bus system shown in Fig.~\ref{fig_2_bus}, in which Bus1 is the PV bus (also the slack bus with $\theta_1=0$) and bus2 is P-Q bus (we fixed $|V_2|=0.9$). We can have the relationship between load and the solution as follows:
% \begin{eqnarray}
%     \label{aceq1}
%     &&P_G=P_D+r\frac{P_{D}^{2}+Q_{D}^{2}}{\left| V_2 \right|^2}, Q_G=Q_D+x\frac{P_{D}^{2}+Q_{D}^{2}}{\left| V_2 \right|^2}, \nonumber \\  
%     \label{aceq3}    
%     &&\left| V_1 \right|=\sqrt{\left| V_2 \right|^2+2rP_D+2xQ_D+\left( r^2+x^2 \right) \frac{P_{D}^{2}+Q_{D}^{2}}{\left| V_2 \right|^2}}, \nonumber \\
%     \label{aceq4}     
%     %&&\theta_2=\arctan \frac{rQ_G-xP_G}{\left| V_1 \right|^2-xQ_G-rP_G}. \nonumber
%     &&\theta _2=\arctan \frac{rQ_D-xP_D}{\left| V_2 \right|^2+rP_D+xQ_D}. \nonumber
% \end{eqnarray}
% It is obvious that the mappings from load ($P_D$ and $Q_D$) to the optimal solution ($P_G$, $Q_G$, $\left| V_1 \right|$ and $\theta_2$) are nonlinear and second-order derivatives exists, which corroborates our analysis in Sec.~\ref{sec:OPF.theory_analysis}. 

% \begin{figure}[t]
% 	\centering
% 	\includegraphics[width = 0.4\textwidth]{../figs/2-bus-example}
% 	\caption{Illustration of 2-bus example.} 
% 	\label{fig_2_bus}
% \end{figure}

\section{Proof of Lemma~\ref{lem3}} \label{lem3_proof}
\begin{proof}
Recall that the load input for the AC-OPF problem by $\mathbf{D}:=\left( P_{Di},Q_{Di},i\in \mathcal{N} \right)$ and the optimal solution as $\mathbf{X}^{*}:=\left( P^{*}_{Gi},Q^{*}_{Gi},|V^{*}_i|,\theta^{*}_i,i\in \mathcal{N} \right)$. The AC-OPF load-solution mapping is denoted by $f^*(\cdot)$, i.e., $\mathbf{X}^{*}=f^*\left( \mathbf{D} \right)$. The AC-OPF problem is essentially a nonlinear programming problem:
\begin{eqnarray}
&\min_{\mathbf{X}}& \,\,c\left( \mathbf{X} \right) \nonumber\\
&\mathrm{s.t.\;\;}&g_i\left( \mathbf{X,D} \right) = 0,\,\,i \in \mathcal{M},\\
&&h_j\left( \mathbf{X} \right) \le 0,\,\,j \in \mathcal{H}, \nonumber
\label{ac.opf.nlp}
\end{eqnarray}
where $c(\cdot)$ is strictly convex function. $\mathcal{M}$ and $\mathcal{H}$ denote the set of equality and inequality constraints. We first have the following corollary using results in~\cite{spingarn1979generic} shows the almost each optimal solution satisfy the following constraints qualifications given the functions $c\left(\cdot \right)$ and $g_i\left( \cdot \right)$ are sufficient smooth:
\begin{corollary} \label{col8}
Except for a set of Lebesgue measure zero, each local optimal solution $\mathbf{X}^{*}$ to the AC-OPF problem satisfies the KKT conditions with strict complementary slackness, linear independence constraint qualification and strongly second-order sufficiency condition.
\end{corollary}
\noindent By leveraging that $c\left(\cdot \right)$ of the AC-OPF problem belong to $C^2$,  $g_i\left(\cdot \right)$ and $h_j\left(\cdot \right)$ of the AC-OPF problem belong to $C^{\infty}$, the above result is obtained by the Sard's theorem~\cite{spingarn1979generic}. We then define the active inequality constraints as follows.
\begin{defi}\label{def1}
    Let $\varPhi$ denote the compact input domain of $\mathbf{D}$. For given $\mathbf{D} \in \varPhi$, the active inequality constraints is defined by
    $$
    \mathcal{A} =\left\{  \left\{j  \right\} |\mathbf{X}^*=f^*\left( \mathbf{D} \right) ,h_j\left( \mathbf{X}^* \right) = 0 \right\}.
    $$
\end{defi}
\noindent For the entire input domain, it could be divided into several regions with different active inequality constraints, which corresponds to multi-element $\mathcal{A}$. With the above conditions in Corollary~\ref{col8} hold, $f^*(\cdot)$ is differentiable in the open subset of each region where the active inequality constraints are unchanged according to the sensitivity analysis and implicit function theorem~\cite{jittorntrum1984solution}. Therefore, the discontinuities only could exist in a set of Lebesgue measure zero (i.e., the boundary of the region).

We below show that the second-order derivative of $\mathbf{X}^*$ w.r.t. $\mathbf{D}$ exists if $f^*(\cdot)$ is differentiable. Let $L=c\left( \mathbf{X}^* \right) +\sum_{i\in \mathcal{M}\,}{\lambda _{i}^{*}g_i\left( \mathbf{X}^*,\mathbf{D} \right)}+\sum_{j\in \mathcal{A}}{\mu _{j}^{*}h_j\left( \mathbf{X}^* \right)}$, where $\lambda_i$ and $\mu_{j}^{'}$ are the corresponding optimal Lagrangian multipliers. We then obtain the first-order Karush Kuhn Tucker (KKT) optimality conditions for~\eqref{ac.opf.nlp} as follows~\cite{pistikopoulos2011multi}:
\begin{eqnarray}
&&\nabla L=0, \nonumber\\
&&g_i\left( \mathbf{X}^*,\mathbf{D} \right) =0,i\in \mathcal{M}; h_j\left( \mathbf{X}^* \right) =0, j\in \mathcal{A}, \nonumber
\label{ac.opf.kkt}
\end{eqnarray}
\noindent Let $\mathbf{Z}=[\mathbf{X}^*;\lambda _{i}^{*},i\in \mathcal{M};\mu_{j}^{*},j\in \mathcal{A}]$. As $f^*\left(\cdot \right)$ is differentiable except for a set of Lebesgue measure zero, we obtain the first-order derivative of $\mathbf{Z}$ w.r.t. $\mathbf{D}$ based on implicit function theorem~\cite{jittorntrum1984solution} as:
\begin{equation}
\frac{d\mathbf{Z}}{d\mathbf{D}}=-A^{-1}B,
\label{first.order.derivative}
\end{equation}
\noindent where
\begin{equation}
A=\left[ \begin{matrix}
	\nabla _{\mathbf{X}^*\mathbf{X}^*}^{2}L&		\nabla _{\mathbf{X}^*}g_1&		...&		\nabla _{\mathbf{X}^*}g_i&		\nabla _{\mathbf{X}^*}h_1&		...&		\nabla _{\mathbf{X}^*}h_j\\
	\left( \nabla _{\mathbf{X}^*}g_1 \right) ^T&		0&		...&		0&		0&		...&		0\\
	...&		...&		...&		...&		...&		0&		...\\
	\left( \nabla _{\mathbf{X}^*}g_i \right) ^T&		0&		...&		0&		0&		...&		0\\
	\left( \nabla _{\mathbf{X}^*}h_1 \right) ^T&		0&		...&		0&		0&		...&		0\\
	...&		...&		0&		...&		...&		0&		...\\
	\left( \nabla _{\mathbf{X}^*}h_j \right) ^T&		0&		...&		0&		0&		...&		0\\
\end{matrix} \right] \nonumber
\end{equation}
and 
\begin{equation}
B=\left[ \begin{array}{c}
	\nabla _{\mathbf{X}^*\mathbf{D}}^{2}L\\
	\left( \nabla _{\mathbf{D}}g_1 \right) ^T\\
	...\\
	\left( \nabla _{\mathbf{D}}g_i \right) ^T\\
	\left( \nabla _{\mathbf{D}}h_1 \right) ^T\\
	...\\
	\left( \nabla _{\mathbf{D}}h_j \right) ^T\\
\end{array} \right].\nonumber
\end{equation}
\noindent where $\nabla _{\mathbf{X}^*} g_i$ and $\nabla _{\mathbf{X}^*} h_j$ denote the gradient of $g_j$ and $h_i$ w.r.t. $\mathbf{X}^*$, respectively. Similarly, $\nabla _{\mathbf{D}} g_i$ and $\nabla _{\mathbf{D}} h_j$ denote the gradient of $g_j$ and $h_i$ w.r.t. $\mathbf{D}$, respectively. Noted that the derivative of $\mathbf{X}^*$ w.r.t. $\mathbf{D}$ can be obtained by elements in the first $2\cdot card{\mathcal{N}}$ row of $-A^{-1}B$, We then obtain the second-order derivative for each $i$-th dimension of $\mathbf{D}$ as follows:
\begin{eqnarray}
\frac{d^2\mathbf{Z}}{d\mathbf{D}_i^2}=A^{-1}\frac{dA}{d\mathbf{D}_i}A^{-1}B_i-A^{-1}\frac{dB_i}{d\mathbf{D}_i}, \nonumber
\end{eqnarray}%-\frac{d\left( M'^{-1}N' \right)}{d\mathbf{D}}
\noindent where $B_i$ denotes the corresponding column in $B$. As the elements in $A$ and $B$ are functions of $\mathbf{X}$, the derivative can be obtained by the results in~\eqref{first.order.derivative}. Therefore, the Hessian of $f^*(\cdot)$ exists. 

% Since $c(\cdot)$ is strictly convex function belongs to class $C^2$ and $g(\cdot)$ are of class $C^{\infty}$, we can obtain the second-order derivative as follows:
% \begin{equation}
% second-order derivative expression
% \end{equation}
% \noindent where xxx.
% Noted that this conclusion holds for the entire domain. Thus, for a compact input domain, the load-solution mapping $f^*(\cdot)$ is a piece-wise smooth function, where each piece belongs to class $C^2$ except for a set of zero-measure points. 

%We further consider the case when convex relaxation is exact, in which the AC-OPF problem is essentially a convex optimization problem with unique optimal solution. Let $S(\mathbf{D})$ denote corresponds to the feasible region given the load $\mathbf{D}$. Suppose $\mathbf{\tilde{D}}$ is the load on the intersection of the segments, we have $\lim_{\mathbf{D}\rightarrow \mathbf{\tilde{D}}}S\left( \mathbf{D} \right) =S\left( \mathbf{\tilde{D}} \right) $. As $S(\mathbf{D})$ is a continuous region due to the convexity of the problem, there exist an arbitrary small open ball $B\left( \mathbf{\tilde{D}} \right)$ such that the intersection between $B \left( \mathbf{\tilde{D}} \right)$ and $S\left( \mathbf{\tilde{D}} \right)$ is not empty. Thus, $\lim_{\mathbf{D}\rightarrow \mathbf{\tilde{D}}}f^*\left( \mathbf{D} \right) =f^*\left( \mathbf{\tilde{D}} \right)$, i.e., the load-generation mapping is continuous at $\mathbf{\tilde{D}}$; otherwise either $f^*\left( \mathbf{\tilde{D}} \right)$ or $f^*\left( \mathbf{D} \right) $ is not the optimal solution. Thus, the mapping $f^*\left( \cdot \right)$ is continuous on the entire input domain. 
\end{proof}

\section{Proof of Theorem~\ref{thm4}} \label{thm4_proof}
\begin{proof}
Suppose $f(\cdot)$ belongs to the class of all the mapping generated by a $n$ neurons deep neural network with ReLU activation function, and is applied to approximate the load-solution mapping $f^*(\cdot)$. Let $p_{\mathbf{D}}$ be the density function of $\mathbf{D}$, and the approximation error is $l_2$-norm error. 

We first shows $f^*(\cdot)$ is measurable on the input domain $\varPhi$. According to Lemma~\ref{lem3}, the load-solution mapping $f^*(\cdot)$ is a continuous except for a set of Lebesgue measure zero. As the continuous function is measurable, we can derive $f^*(\cdot)$ is measurable by definition of measurable function, $f^*(\cdot)$ is measurable. Based on Lusin's Theorem~\cite{royden1988real}, for each $\varepsilon > 0$ there exists a continuous function $f'(\mathbf{D})$ and a set $\varPhi' \subseteq \varPhi$ such that:
\begin{equation}
\varPhi' =\left\{ \mathbf{D|}f'\left( \mathbf{D} \right) \ne f^{*}\left( \mathbf{D} \right) \right\} \,\,\mathrm{and\,\,}\phi\left(\varPhi'\right) <\varepsilon,
\label{lusin.theorem}
\end{equation}
\noindent where $\phi\left( A \right)$ represent the measure of set $A$. We then expand the approximation error as follows:
\begin{eqnarray}
&&E_{\mathbf{D}\backsim p_{\mathbf{D}}}\left[ \left( f^*\left( \mathbf{D} \right) -f\left( \mathbf{D} \right) \right) ^2 \right] \nonumber\\%\lim_{n\rightarrow \infty}
&=&E_{\mathbf{D}\backsim p_{\mathbf{D}}}\left[ \left( f^*\left( \mathbf{D} \right) -f'\left( \mathbf{D} \right) +f'\left( \mathbf{D} \right) -f\left( \mathbf{D} \right) \right) ^2 \right]  \nonumber\\%\lim_{n\rightarrow \infty}
&\le& E_{\mathbf{D}\backsim p_{\mathbf{D}}}\left[ \left( f^*\left( \mathbf{D} \right) -f'\left( \mathbf{D} \right) \right) ^2 \right] \nonumber \\%\lim_{n\rightarrow \infty}
&&+E_{\mathbf{D}\backsim p_{\mathbf{D}}}\left[ \left( f'\left( \mathbf{D} \right) -f\left( \mathbf{D} \right) \right) ^2 \right]. \nonumber%\lim_{n\rightarrow \infty}
\label{approximation.error1}
\end{eqnarray}
\noindent The error consists of two parts, where the first term relies on the expected square error between $f'\left( \cdot \right)$ and $f^*\left( \mathbf{D} \right)$ on the input domain (independent of DNN model) and the second term depends on the approximation error using DNN to approximation $f'\left( \cdot \right)$. We first have:
\begin{eqnarray}
&&\lim_{n\rightarrow \infty}E_{\mathbf{D}\backsim p_{\mathbf{D}}}\left[ \left( f^*\left( \mathbf{D} \right) -f'\left( \mathbf{D} \right) \right) ^2 \right] \nonumber\\
&\le& \max_{\mathbf{D}\in \varPhi'}\left( f^*\left( \mathbf{D} \right) -f'\left( \mathbf{D} \right) \right) ^2\cdot \phi\left(\varPhi' \right).
\label{error.2nd.part}
\end{eqnarray}
\noindent Since $f^*\left( \cdot \right)$ and $f'\left( \cdot \right)$ are bounded on the input domain $\varPhi$, thus $\max_{\mathbf{D}\in \varPhi'}\left( f^*\left( \mathbf{D} \right) -f'\left( \mathbf{D} \right) \right) ^2$ is bounded and can be regarded as a constant. By~\eqref{lusin.theorem}, the error in~\eqref{error.2nd.part} can be arbitrarily small. As $f'\left( \mathbf{D} \right)$ is continuous, based on the universal approximation theorem, i.e., there is an $n_{\epsilon}$, so that for any $n \ge n_{\epsilon}$, there exists an $f(\cdot)\in \mathcal{K}_n$ such that the $E_{\mathbf{D}\backsim p_{\mathbf{D}}}\left[ \left( f'\left( \mathbf{D} \right) -f\left( \mathbf{D} \right) \right) ^2 \right]$ is arbitrarily small. Consequently, we derive~\eqref{universial.approximation.acopf}.
% for each $\epsilon >0$, there exists an $f(\cdot)$ generated by DNN with $n$ neurons and $n>\epsilon_N$ such that 
%\begin{equation}
%E_{\mathbf{D}\backsim p_{\mathbf{D}}}\left[ \left( f^*\left( \mathbf{D} \right) -f\left( \mathbf{D} \right) \right) ^2 \right]<\epsilon.%\lim_{n\rightarrow \infty}
%\end{equation}
\end{proof}

% \section{Proof of Theorem~\ref{thm6}}
% \label{apx:thm:approximation-error}
% \begin{proof}
% Suppose $\mathcal{K}$ is the class of all $f(\cdot)$ generated by a DNN with $L$ hidden layers and at most $m$ neurons per layer. Recall that $\varPhi = \left[ \text{0,}\text{1} \right]^{\text{2*card}\left( \mathcal{N} \right)}$, and $\mathbf{D}$ obeys the uniform distribution on $\varPhi $ with density function $u_{\mathbf{D}}$. According to Appendix~\ref{thm4_proof}, there exists a set $\varPhi'$ ($ \varPhi'\subseteq \varPhi, \phi(\varPhi)>0$), on which $f(\mathbf{D})$ is continuous and with non-zero Hessian. We have the following equations by only considering the approximation error on $\varPhi'$:
% \begin{eqnarray}
% &&E_{\mathbf{D}\backsim u_{\mathbf{D}}}\left[ \left( f^*\left( \mathbf{D} \right) -f\left( \mathbf{D} \right) \right) ^2 \right]  \nonumber\\
% &\ge& E_{\mathbf{D}\backsim u_{\mathbf{D}},\mathbf{D}\in \varPhi'}\left[ \left( f^*\left( \mathbf{D} \right) -f\left( \mathbf{D} \right) \right) ^2 \right], \nonumber\\
% &=&\Omega \left( \frac{1}{\left( 2m \right) ^{4L}} \right),\nonumber
% \label{approximation.error.lower.bound}
% \end{eqnarray}
% \noindent where the last inequality is obtained using result in~\cite{SafranS17} (Theorem. 7) on approximating twice-differentiable function with DNN.
% % \begin{corollary} \label{col8}
% % Let $x$ obeys the uniform distribution on $\left[ \text{0,}\text{1} \right]^{d}$. Suppose $\mathcal{K}$ is the class of all $f(\cdot)$ generated by a DNN with $L$ hidden layers and at most $m$ neurons per layer. For a given a twice-differentialable function $\eta(\cdot)$, we have following bound for $\forall f(\cdot) \in \mathcal{K}$.
% % \begin{equation}
% % E_{_{x\backsim u_{\mathbf{D}}}}\left[ \left(\eta\left( x\right) -f\left( x \right) \right) ^2 \right] = 
% % \label{lower.bound.ac}
% % \end{equation}
% % \end{corollary}
% Plugging the relationship into~\eqref{lower.bound.ac}, we have the same result in Theorem~\ref{thm6}.
% \end{proof}

% \section{Proof of Corollary~\ref{col7} } \label{apx:proof_of_col1}
% \begin{proof}
% We next will show how to derive the Corollary \ref{col7}. 
% Suppose $\epsilon$ is defined as the upper bound for the $l_2$-norm approximation error:
% \begin{equation}
% E_{\mathbf{D} \backsim \mu_{\varPhi}}\left[ \left( f^*\left( \mathbf{D} \right) -f\left( \mathbf{D} \right) \right) ^2 \right] \le \epsilon
% \end{equation}
% Then, we can derive the following inequality based on the above definition and Theorem \ref{thm6}:
% \begin{equation}
% \epsilon \geq \frac{c}{\left( 2m \right) ^{4L}},
% \end{equation}
% \noindent where $c$ is a constant. We then can obtain the following necessary condition related to the DNN's size provided on the Corollary \ref{col7}:
% \begin{equation}
% \left( 2m \right) ^{4L} = \Omega \left( \frac{1}{\epsilon} \right).
% \end{equation}
% \end{proof}

\end{appendices}



% % \begin{figure}[!t]
% % 	\centering
% % 	\includegraphics[width = 0.45\textwidth]{../figs/lemma2}
% % 	\caption{Illustration of approximating a two-segment piece-wise Lipschitz-continuous function $h(\cdot)$ by a linear function $g(\cdot)$.} 
% % 	\label{fig_appro}
% % \end{figure}

% %\appendix      

% %%%%%% for the next  appendix section
% %%% commented out for smooth previewing the PDF output, Feb. 2, 2019
% %%%%%%
% \section{Proof of Lemma~\ref{lem1}} \label{lem1_proof}
% \begin{proof}
% We now show the considered piece-wise linear one-dimension output function $f^*(\cdot)$ is Lipschitz-continuous in the input domain $\mathcal{D}$, which can be partitioned into $r$ different convex polyhedral regions, ${R}_i,i=1,...,r$. The mapping $f^{*}\left( \cdot \right)$ is  piece-wise linear and  can be defined as follows: 
%  \begin{equation*}
%      f^{*}\left( x \right)=
%      \begin{cases}
%      a_1 x + b_1, \ \textrm{if} \ x \in {R}_1\\
%      a_2 x + b_2, \ \textrm{if} \ x \in {R}_2\\
%      \cdots \\
%      a_r x + b_r, \ \textrm{if} \ x \in {R}_r\\
%      \end{cases}
%  \end{equation*}
% where $x \in \mathbf{R}^{n \times 1}, a_i \in \mathbf{R}^{1 \times n}, i=1,...,r $ and $b_i \in \mathbf{R}^{1}, i=1,...,r $. Then, we can have:\rev{
%  \begin{equation}
%  \begin{aligned}
%  \left| f^{*}\left( x_1 \right) -f^{*}\left( x_2 \right) \right| \le \lVert a_i \rVert \cdot \lVert x_1-x_2 \rVert, \forall x_1,x_2 \in \mathcal{D}. \nonumber
%  \end{aligned}
%  \end{equation}
%  Thus, let  $ \varLambda = \max\left\{ \lVert a_i \rVert, \dots, \lVert a_r \rVert \right\}$. We have
%  \begin{equation}
%  \begin{aligned}
%  \left| f^{*}\left( x_1 \right) -f^{*}\left( x_2 \right)  \right| \le \varLambda \cdot \lVert x_1-x_2 \rVert \forall x_1,x_2 \in \mathcal{D}.\nonumber
%  \end{aligned}
%  \end{equation}
% }Therefore, $f^{*}\left( \cdot \right)$ is Lipschitz-continuous.
% \end{proof}



% \section{Proof of Lemma~\ref{lem3}} \label{apx:proof_of_lemma_3}

% \begin{proof}\label{proof5}
% We can derive the lower bound to the worst-case $L_{\infty}$-based approximation error as follows. Suppose we want to find a function $g \left( \cdot \right)$ belongs to the linear scalar function class $\mathcal{G}$ to approximate the function $h$ belongs to the two-segment piece-wise linear function class $\mathcal{H}$ with a Lipschitz constant $\varLambda > 0$, over an interval $\left[-\mu,\mu \right]$ ($\mu>0$). An illustration is shown in Fig.~\ref{fig_appro}. Let ${g\left( x \right)}=a\cdot x+b$, for ${x\in \left[ -\mu, \mu \right]}$. Let $\hat{h} \in \mathcal{H}$ be the following:
% \begin{equation}
%     \hat{h} \left(x \right)=
%     \begin{cases}
%     \varLambda (x+\mu), \ \textrm{if} \ x \in \left[-\mu,0 \right]\\
%     -\varLambda (x-\mu), \ \textrm{if} \ x \in \left[0, \mu \right]\\
%     \end{cases}
% \end{equation}

% % Then, we need to show that
% % \begin{equation}
% % \underset{x\in \left[-\mu ,\mu \right]}{\max}\left| \hat{h}\left( x \right) -g\left( x \right) \right| \geq \varLambda \cdot \frac{\mu}{2},\ \mathrm{for}\ \forall \ g\in \mathcal{G}
% % \end{equation}
% Then, we can obtain the lower bound for the $L_{\infty}$-based approximation error of $\hat{h} \left( \cdot \right)$ and $g\left( \cdot \right)$ by the classification discussion on the intercept $b$.
% \begin{itemize}
% \item If $b \le \frac{\varLambda \mu}{2}$. Under this case, we can get: 
% \begin{eqnarray*}
% % &&\underset{x\in \left[-\mu ,\mu \right]}{\max}\left| \hat{h}\left( x \right) -g\left( x \right) \right|\\
% \underset{x\in \left[-\mu ,\mu \right]}{\max}\left| \hat{h}\left( x \right) -g\left( x \right) \right|&\geq& \left| \hat{h}\left( 0 \right) -g\left( 0 \right) \right|\\
% &\geq& \varLambda \cdot \frac{\mu}{2n}\\
% &=&\left| \varLambda \mu -b \right|\\
% &\geq& \varLambda \cdot \frac{\mu}{2}.
% \end{eqnarray*}

% \item Otherwise $\frac{\varLambda \mu}{2}< b $. If $a>0$, under this case we can have:
% \begin{eqnarray*}
% % &&\underset{x\in \left[-\mu ,\mu \right]}{\max}\left| \hat{h}\left( x \right) -g\left( x \right) \right|\\
% \underset{x\in \left[-\mu ,\mu \right]}{\max}\left| \hat{h}\left( x \right) -g\left( x \right) \right|&\geq& \left| \hat{h}\left( \mu \right) -g\left( \mu \right) \right|\\
% &\geq& \left( \varLambda +a \right) \cdot \frac{\mu}{2}\\
% &\geq& \varLambda \cdot \frac{\mu}{2}.
% \end{eqnarray*}
% Otherwise \rev{$a\leq 0$}, we can consider the point $x=-\mu$ and obtain the same result.
% \end{itemize}
% Thus overall, we observe
% \begin{equation}
% \underset{g\in \mathcal{G}}{\min}\ \underset{x\in \left[-\mu ,\mu \right]}{\max}\left| \hat{h}\left( x \right) -g\left( x \right) \right|\geq \varLambda \cdot \frac{\mu}{2}.\nonumber
% \end{equation}
% For the worst-case $L_{\infty}$-based approximation error, we have \rev{
% \begin{align}
%     & \underset{h\in \mathcal{H}}{\max}\ \underset{g\in \mathcal{G}}{\min}\ \underset{x\in \left[-\mu ,\mu \right]}{\max}\left| h\left( x \right) -g\left( x \right) \right| \nonumber \\
%     \geq& \underset{g\in \mathcal{G}}{\min}\ \underset{x\in \left[-\mu ,\mu \right]}{\max}\left| \hat{h}\left( x \right) -g\left( x \right) \right| \nonumber \\
%     \geq& \varLambda \cdot \frac{\mu}{2} \nonumber
% \end{align}
% }
% \end{proof}


% %\section{Proof of Theorem.~\ref{the1}} \label{apx:proof_of_theory_1}
% %\begin{proof}
% %According to Lemma.\ref{lem2}, the mapping $\mathcal{F}\left( \mathbf{P}_{\mathbf{D}} \right)$ is continuous. In addition, $\mathbf{P}_{\mathbf{D}}\in Z$ and $Z$ is a compact set. Lemma. \ref{lem3} shows that any continuous functions on an compact set can be approximated well by a neural network with ReLU as activation function. Thus, the vector-valued mapping can be approximated well by neural network.
% %\end{proof}



% \section{Proof of Theorem~\ref{thm:worst-cast-approximation-error}} \label{apx:proof_of_theory_1}
% \begin{proof}
% We can characterize the lower bound on the worst-case error of using neural networks to approximate load-to-generation mappings in SC-DCOPF problems as follows. 

% Suppose $\mathcal{G}$ be the family of piece-wise linear function class generated by a neural network with depth $N_{\mbox{hid}}$ and maximum number of neurons per layer $N_n$, on the load input domain $\mathcal{D}$ with the diameter $d$. \rev{The maximal number of segment any functions belongs to $\mathcal{G}$ can have is defined as $n$.} %\com{Is this sentence a statement or a definition of $n$?} 
% Let $\mathcal{H}$ be the class of all possible $f^*(\cdot)$ with a Lipschitz constant $\varLambda>0$. \rev{Let $\hat{f} \in \mathcal{H}$ comprises of $2n$ linear segments with equal length be the following:}
% %\com{This statement is not clear. Why there must be $2n$ segments, why they must be equal length?} 
% \begin{equation*}
%     \hat{f} \left(x \right)=
%     \begin{cases}
%     \varLambda (x-a_i), \ \textrm{if} \ x \in \left[a_i,a_{i+1} \right];\\
%     -\varLambda (x-a_{i+2}), \ \textrm{if} \ x \in\left[a_{i+1},a_{i+2} \right].\\
%     \end{cases}
% \end{equation*}
% \rev{where $\left\{ \lVert a_0-a_1 \rVert, ...,  \lVert a_{2i-1}-a_{2i}, i=1,...,n \rVert \right\}=\frac{d}{2n}$}.
% %Let $f \in \mathcal{G}$ be linear when restricted to any interval $\left[a_{i} ,a_{i+2} \right]$. 
% %\com{No clear...}
% %$f_i\left( x \right) =w_ix+z_i, i = 1,...,n$ denote the linear restriction of $f$ to the interval $\left[a_{i} ,a_{i+1} \right]$. 
% According to Lemma \ref{lem3}, on the interval $\left[a_i,a_{i+2} \right], i=0,...,2n-2$, we can have:
% \begin{eqnarray*}
% &&\underset{f\in \mathcal{G}}{\min}\ \underset{x\in \left[ a_i,a_{i+2} \right]}{\max}\left| \hat{f}\left( x \right) -f\left( x \right) \right| \geq \varLambda \cdot \frac{d}{4n}.\\
% %&\geq& \varLambda \cdot \frac{d}{4n}
% \end{eqnarray*}
% Thus,
% \begin{eqnarray*}
% &&\underset{f^{*}\in \mathcal{H}}{\max}\,\, \underset{f\in \mathcal{G}}{\min}\ \underset{x\in \left[ a_i,a_{i+2} \right]}{\max}\left| f^{*}\left( x \right) -f\left( x \right) \right| \geq \varLambda \cdot \frac{d}{4n}.\\
% %&\geq& \varLambda \cdot \frac{d}{4n}
% \end{eqnarray*}

% Meanwhile, we use the result in \cite{telgarsky2016benefits}, of which the following is an immediate corollary:
% \begin{corollary}
% The maximal number of \rev{linear} segments generated from the family of ReLU neural networks with depth \rev{(the number of hidden layers)} $l$ and maximal width (neurons on the hidden layer) $m$ is $\left( 2m \right) ^l$.
% \end{corollary}

% By the above corollary, we have $n\leq \left(2N_n\right)^{N_{\mbox{hid}}}$. Consequently,
% \begin{equation}
% \underset{f^*\in \mathcal{H}}{\max}\ \underset{f\in \mathcal{G}}{\min}\ \underset{x\in \mathcal{D}}{\max}\left| f^*\left( x \right) -f\left( x \right) \right|\geq \varLambda \cdot \frac{d}{4\cdot(2N_n)^{\rev{N_{\mbox{hid}}}}}.
% \end{equation}
% \end{proof}

% \section{Proof of Corollary~\ref{col1} } \label{apx:proof_of_col1}
% \begin{proof}
% We next will show how to derive the Corollary \ref{col1}. Suppose $\epsilon$ is defined as the upper bound for the worst-case approximation error, that is:
% \begin{equation}
% \underset{f^*\in \mathcal{H}}{\max}\,\,\underset{f \in \mathcal{G}}{\min}\ \underset{x\in \mathcal{D}}{\max}\left| f^*\left(x\right) -f\left( x \right) \right|\le \epsilon
% \end{equation}
% Then, we can derive the following inequality based on the above definition and Theorem \ref{thm:worst-cast-approximation-error}:
% \begin{equation}
% \varLambda \cdot \frac{d}{4\cdot(2N_n)^{N_{\mbox{hid}}}} \le \epsilon,
% \end{equation}
% After some transformations, we can obtain the following necessary condition related to the DNN's scale on the Corollary \ref{col1}, which can guarantee that the designed DNN's ever possible to approximate the most difficult load-to-generation mapping with a Lipschitz constant $\varLambda$, up to an error of $\epsilon>0$:
% \begin{equation}
% (2N_n)^{N_{\mbox{hid}}}\geq \varLambda \cdot \frac{d}{4\cdot \epsilon}.
% %\label{err_bound_dnn2}
% \end{equation}
% \end{proof}
% %\com{to be continued...? A: I will do it soon.} 

% \section{Proof of Proposition~\ref{prop:DeepOPF.complexity} } \label{apx:proof_of_prop5}
% \begin{proof}
% We next will show how to derive the computational complexity \rev{of using the DNN model to obtain the generation output from the given input}. Recall that the input and the output of the DNN model in \textsf{DeepOPF} are $N_{\mbox{in}}$ and $N_{\mbox{out}}$ dimensions, respectively, and the DNN model has $N_{\mbox{hid}}$ hidden layers and each hidden layer has $N_{\mbox{i}}$, $i=1,...,N_{\mbox{hid}}$. The maximal neurons on the hidden layers is $N_{n}$ neurons. For each neuron in the DNN model, we can regard the computation complexity on each neuron (measured by basic arithmetic operation) as $\mathcal{O} \left(1\right)$. As we apply the fully-connected architecture, the output of each neuron is calculated by taking a weighted sum of the output from the neurons on the previous hidden layer and passing through a activation function.

% Thus, the computational complexity (measured as the number of arithmetic operations) to generate the output from the input by a DNN model consists of the following three parts:
% \begin{itemize}
% \item Complexity of computation from the input to the first hidden layer. As each neuron on the first hidden layer will take the input data, thus the corresponding complexity  is $\mathcal{O} \left(N_{\mathrm{in}}N_1\right)$.

% \item Complexity of computation between the consecutive hidden layers. Since each neuron on the current hidden layer will take the output from each neuron on the previous hidden layer as the input data. Thus, thus the corresponding complexity is $\mathcal{O} \left(\sum_{i=1}^{N_{\mathrm{hid}}-1}{N_iN_{i+1}}\right)$.

% \item Complexity of computation from the last hidden layer to the output. As the output of each neuron on the last hidden layer is used to calculated the output, the corresponding complexity is $\mathcal{O} \left(N_{hid}N_{out}\right)$.
% \end{itemize}

% Hence, the whole complexity of the calculation by a DNN model is:
% \begin{eqnarray*}
% %T&=&N_{\mathrm{in}}N_1+\sum_{i=1}^{N_{\mathrm{hid}}-1}{N_iN_{i+1}}+N_{hid}N_{out}\\
% T&=&\mathcal{O}\left( N_{\mathrm{in}}N_1+N_{\mathrm{hid}}N_{\mathrm{n}}^{2}+N_{hid}N_{out} \right)\\
% &=&\mathcal{O}\left( N_{\mathrm{hid}}N_{\mathrm{n}}^{2} \right).\\
% \end{eqnarray*}
% \end{proof}
